# Supplementary material for: MCBeth: A Measurement Based Quantum Programming Language
Source: arXiv:2204.10784 source file (2022-06-25)
Supplement: Supplementary file 1 [file supplemental.tex]

%% For double-blind review submission, w/o CCS and ACM Reference (max submission space)
\documentclass[acmsmall,review, anonymous]{acmart}\settopmatter{printfolios=true,printccs=false,printacmref=false}
\settopmatter{printfolios=true,printccs=false,printacmref=false}

%% Citations
% \usepackage{biblatex} % Removed, since acmart seems to use natbib which conflicts
% \addbibresource{cites.bib}
\usepackage{cleveref}
\usepackage{stmaryrd}
\usepackage{alltt}
\usepackage{graphicx}
\graphicspath{{./figures/}{../figures/}}

\usepackage{semantic}
\usepackage{adjustbox}

% Color
\usepackage{bcprules}
\usepackage{backnaur}
\usepackage{pgfplots}
\usepackage{tikz}
\usepackage{multirow}

\usepackage{algorithm}
\usepackage[noend]{algpseudocode}

\usepackage[frame,line,arrow,matrix,tips]{xy}	% all that is usually necessary

%%%%%%%%%%%%%%%%%%%%%%%%%%%%%%%%%%%%%%%%%%%%%%%%%%%%%%%%%%%%%%%%%%%%%%%%%%%%%
% For OCAML
\usepackage{minted}
\usepackage[T1]{fontenc}
\usepackage{textcomp}
\usepackage[scaled]{beramono}

\usepackage{listings}

\definecolor{codegreen}{rgb}{0,0.6,0}
\definecolor{codegray}{rgb}{0.5,0.5,0.5}
\definecolor{codepurple}{rgb}{0.58,0,0.82}
\definecolor{backcolour}{rgb}{0.95,0.95,0.92}

\lstdefinestyle{MCBethStyle}{            
    backgroundcolor=\color{backcolour},   
    commentstyle=\color{codegreen},
    keywordstyle=\color{magenta},
    numberstyle=\tiny\color{codegray},
    stringstyle=\color{codepurple},
    basicstyle=\small\ttfamily,
  breakatwhitespace=false,
  breaklines=true,
  captionpos=b,
  keepspaces=true,
  numbers=none,              
    numbersep=5pt,                  
    showspaces=false,                
    showstringspaces=false,
    showtabs=false,                  
    tabsize=2
  float=ht,
  frame=tb,
}

%%%%%% Setup for Quantum Circuit Diagram Creation %%%%%%
\CompilePrefix{xygui-}

%%%%%%%%%%%%%%%%%%%%%%%%%%%%%%%%%%%%%%%%%%%%%%%%%%%%%%%%%%%%%%%%%%%%%%%%%%%%%
% wires

\def\w{\ar@{-}[l]}
\def\W{\ar@{=}[l]}

%%%%%%%%%%%%%%%%%%%%%%%%%%%%%%%%%%%%%%%%%%%%%%%%%%%%%%%%%%%%%%%%%%%%%%%%%%%%%
% labels

% simple label

%%%%%%%%%%%%%%%%%%%%%%%%%%%%%%%%%%%%%%%%%%%%%%%%%%%%%%%%%%%%%%%%%%%%%%%%%%%%%
% single qubit operations

	% operator in box

				% for swap gate
			% square, for controlled-phase
		% matrix shortcut
	% re-init to |0>
	% vertical ``|''
				% slash for wire bundles

%%%%%%%%%%%%%%%%%%%%%%%%%%%%%%%%%%%%%%%%%%%%%%%%%%%%%%%%%%%%%%%%%%%%%%%%%%%%%
% nop's

%%%%%%%%%%%%%%%%%%%%%%%%%%%%%%%%%%%%%%%%%%%%%%%%%%%%%%%%%%%%%%%%%%%%%%%%%%%%%
% misc definitions

\def\>{\rangle}
\def\<{\langle}

% measurement box
\def\meter{*+[]{\put(-4,0){\includegraphics[scale=.5]{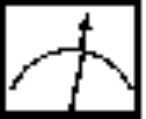}}\hspace{14pt}}%
		\ar@{-}[l]}

%%%%%%%%%%%%%%%%%%%%%%%%%%%%%%%%%%%%%%%%%%%%%%%%%%%%%%%%%%%%%%%%%%%%%%%%%%%%%
% qubit names (and also revert to qubit wires, vs, cbit wires)

%%%%%%%%%%%%%%%%%%%%%%%%%%%%%%%%%%%%%%%%%%%%%%%%%%%%%%%%%%%%%%%%%%%%%%%%%%%%%
% multiple qubit gates

% empty space of width determined by the text argument
\def\gspace#1{*+{\rule[-0.2ex]{0ex}{2.1ex}%
	\setbox\sbox=\hbox{$#1$}%
	\hspace*{\wd\sbox}}}
	
% n-qubit operation #1=box label, #2=number of qubits (eg d=2 qubits, ddd=4)

% two-qubit operation

% two-qubit operation

%%%%%%%%%%%%%%%%%%%%%%%%%%%%%%%%%%%%%%%%%%%%%%%%%%%%%%%%%%%%%%%%%%%%%%%%%%%%%
% ``D'' style measurement gate a-la-cleve, at Michael Nielsen's request

%%%%%%%%%%%%%%%%%%%%%%%%%%%%%%%%%%%%%%%%%%%%%%%%%%%%%%%%%%%%%%%%%%%%%%%%%%%%%

%% Journal information
%% Supplied to authors by publisher for camera-ready submission;
%% use defaults for review submission.
\acmJournal{PACMPL}
\acmVolume{1}
\acmNumber{OOPSLA} % CONF = POPL or ICFP or OOPSLA
\acmArticle{1}
\acmYear{2018}
\acmMonth{1}
\acmDOI{} % \acmDOI{10.1145/nnnnnnn.nnnnnnn}
\startPage{1}

%% Copyright information
%% Supplied to authors (based on authors' rights management selection;
%% see authors.acm.org) by publisher for camera-ready submission;
%% use 'none' for review submission.
\setcopyright{none}
%\setcopyright{acmcopyright}
%\setcopyright{acmlicensed}
%\setcopyright{rightsretained}
%\copyrightyear{2018}           %% If different from \acmYear

%% Citation style
%% Note: author/year citations are required for papers published as an
%% issue of PACMPL.
\citestyle{acmauthoryear}   %% For author/year citations

%%%%%%%%%%%%%%%%%%%%%%%%%%%%%%%%%%%%%%%%%%%%%%%%%%%%%%%%%%%%%%%%%%%%%%
%% Note: Authors migrating a paper from PACMPL format to traditional
%% SIGPLAN proceedings format must update the '\documentclass' and
%% topmatter commands above; see 'acmart-sigplanproc-template.tex'.
%%%%%%%%%%%%%%%%%%%%%%%%%%%%%%%%%%%%%%%%%%%%%%%%%%%%%%%%%%%%%%%%%%%%%%

\title{MCBeth Supplementary Material}

\begin{document}
\maketitle

%% Note: \maketitle command must come after title commands, author
%% commands, abstract environment, Computing Classification System
%% environment and commands, and keywords command.
\section{Software Artifact}
All software created for this work is available via an anonymous opensource repository: \url{https://anonymous.4open.science/r/mcbeth-728B/}. 

\section{Cluster States}
\input{blocks.tex}

\section{Side by side code comparison}
\input{codecomparison.tex}

\end{document}
